# Supplementary material for: What, when, and where? -- Self-Supervised Spatio-Temporal Grounding in Untrimmed Multi-Action Videos from Narrated Instructions
Source: arXiv:2303.16990 source file (2024-05-28)
Supplement: Supplementary file 2 [file eval.tex]

\begin{figure*}[t]
    \centering
    \includegraphics[width=\textwidth]{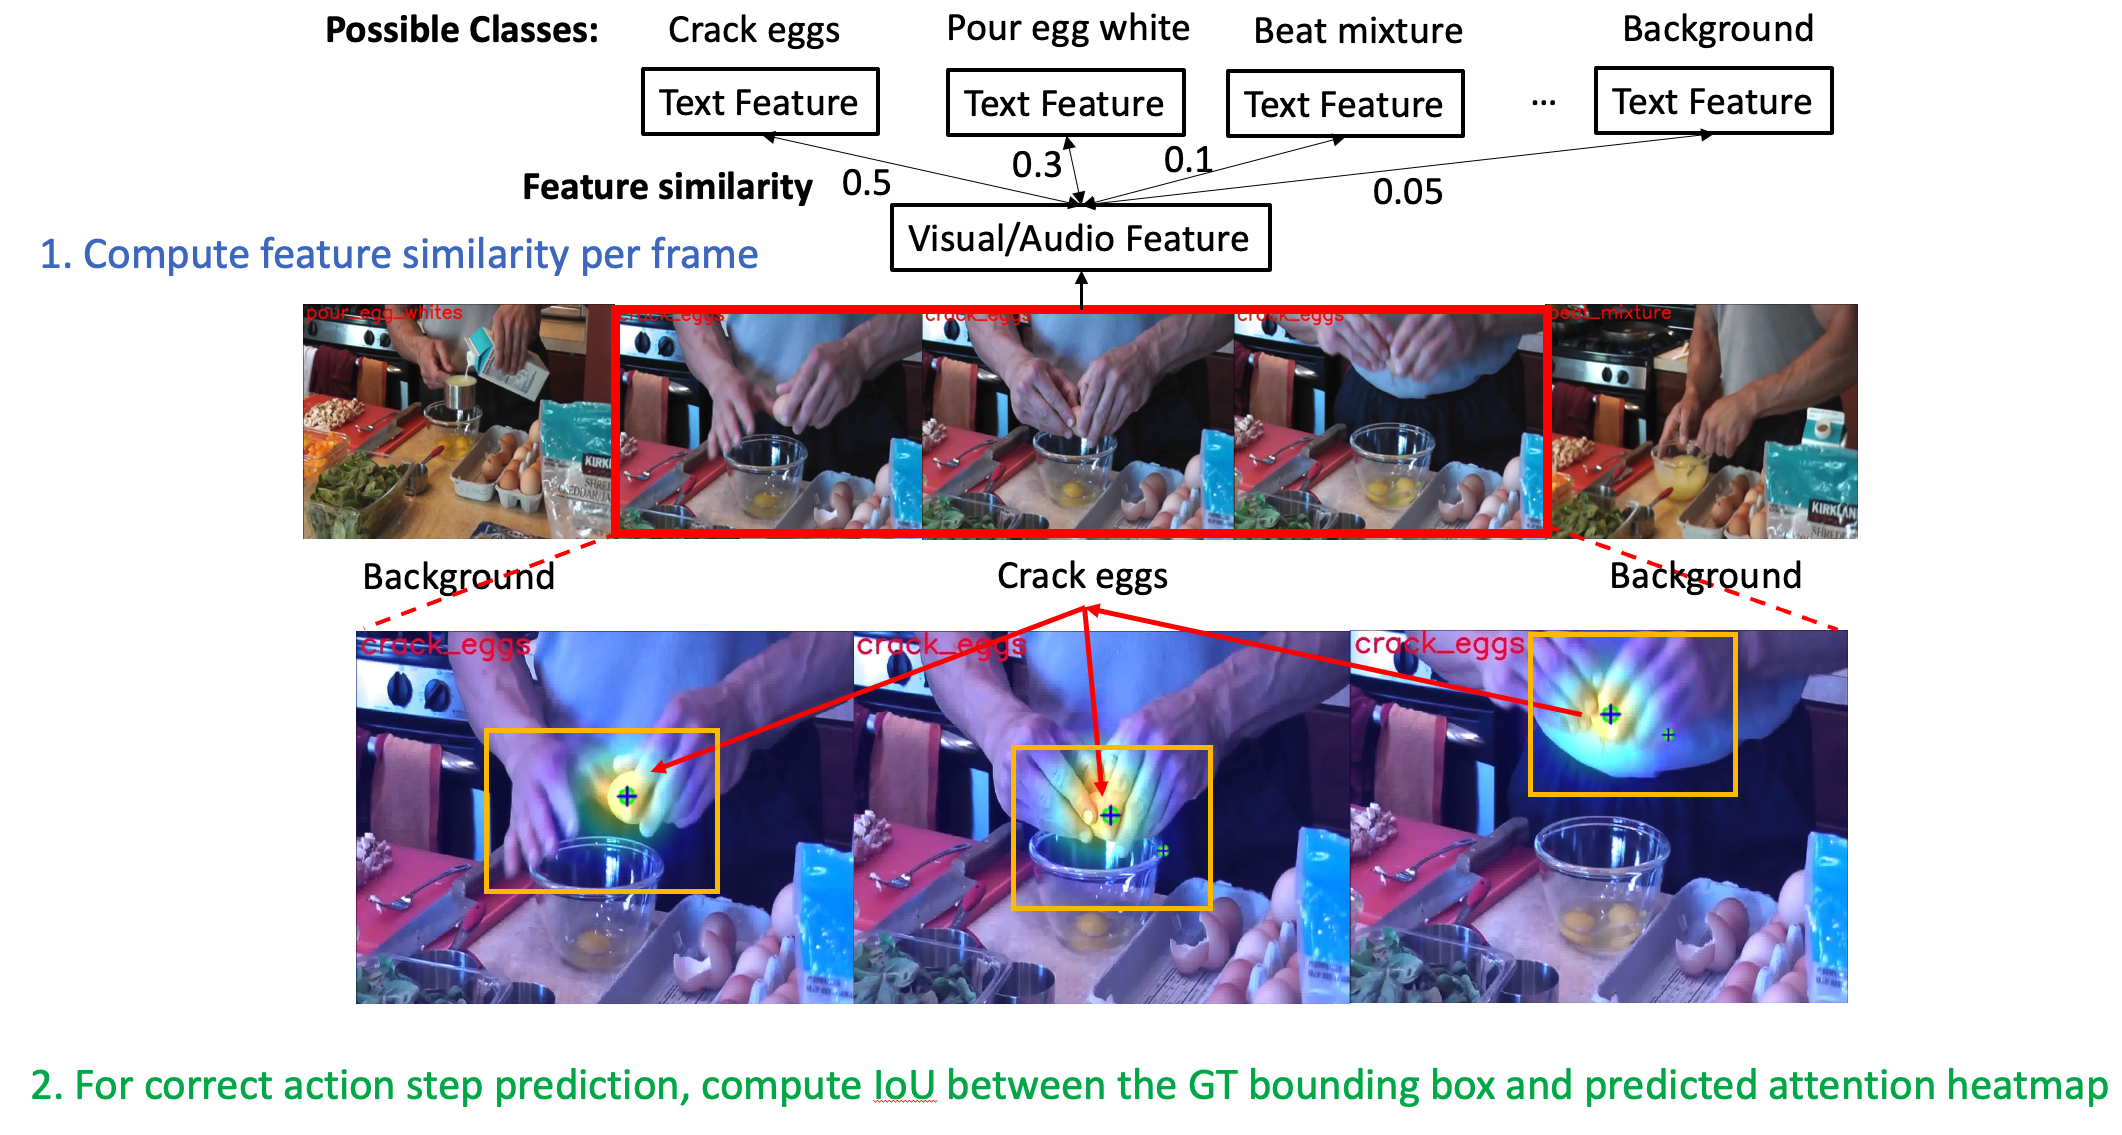}
    
    \caption{\textbf{Multimodal Spatio-temporal Grounding Evaluatation pipeline (Clip level).} We start by localizing the start time and end time of the action step in the video using feature similarity between video/audio features and text features. We select the action class with the maximum probability. Given the frames with a correct prediction, we check the IoU between the GT box and the predicted attention heatmap by the model. The prediction is correct when both labels are correct, and the IoU surpasses a certain threshold.}%\bc{This is directly modified by MCN, will modify the figure soon}}
    \label{fig:eval}
    \vspace{-10pt}
\end{figure*}
