# Supplementary material for: What, when, and where? -- Self-Supervised Spatio-Temporal Grounding in Untrimmed Multi-Action Videos from Narrated Instructions
Source: arXiv:2303.16990 source file (2024-05-28)
Supplement: Supplementary file 4 [file loss.tex]

\begin{table}[h]
        \centering%\vspace*{1mm}
		 \begin{tabularx}{0.45\linewidth}{lp{3em}c}
			\toprule
				\multirow{2}{*}{\textbf{Loss}} & & mAP  \\
					  & & IOU@0.4 \\
				\hline
				CoMMA* \cite{tan2021look}  &  &   2.65 \\
				MIL-NCE \cite{miech2020end} &  &   3.71 \\
				\midrule
				w/o $L_{Global}$ loss                          &  &   2.61 \\
				w/o $L_{Local}$ loss                      &  &   4.10 \\
				Ours                         &  &   20.29 \\ 
			%\midrule
			\bottomrule
		\end{tabularx}
		\vspace{+0.5cm}
		\caption{Ablation on global and local losses. \label{tab:ablation_GL_loss}}
\end{table}
