# Supplementary material for: What, when, and where? -- Self-Supervised Spatio-Temporal Grounding in Untrimmed Multi-Action Videos from Narrated Instructions
Source: arXiv:2303.16990 source file (2024-05-28)
Supplement: Supplementary file 5 [file visualization.tex]

\section{Annotation Visualization Videos}
We include more visualizations of our annotated MiningYoutube Grounding dataset in video format at {\color{blue}\textbf{sup/Annotation visualization videos.pptx}}.
