# Supplementary material for: What, when, and where? -- Self-Supervised Spatio-Temporal Grounding in Untrimmed Multi-Action Videos from Narrated Instructions
Source: arXiv:2303.16990 source file (2024-05-28)
Supplement: Supplementary file 6 [file visual_old.tex]

\begin{figure*}[h]
    \centering
    \begin{subfigure}[h]{\textwidth}
    \centering
    \includegraphics[width=\textwidth]{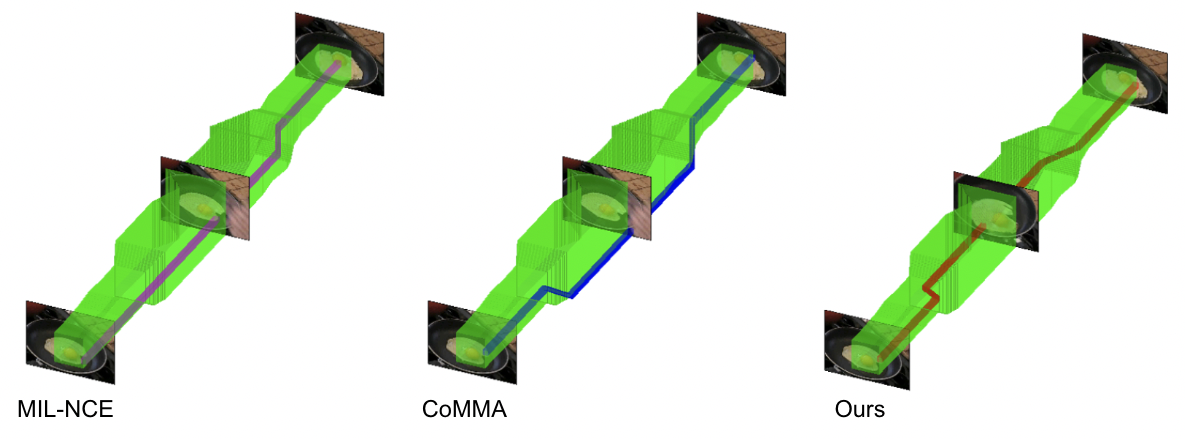}
    %\vspace{-16pt}
    \caption{Frying egg.}
    \label{fig:eval1}
    %\vspace{-1pt}
    \end{subfigure}
    \begin{subfigure}[h]{\textwidth}
    \centering
    \includegraphics[width=\textwidth]{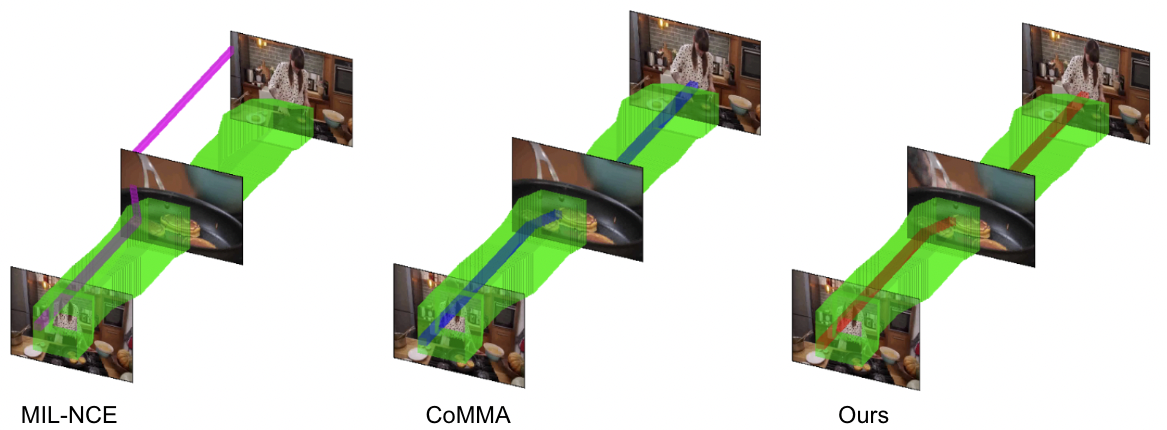}
    %\vspace{-16pt}
    \caption{Flip pancake.}
    \label{fig:eval1}
    %\vspace{-1pt}
    \end{subfigure}
    
    
    %\bc{This is directly modified by MCN, will modify the figure soon}}
    %\label{fig:eval}
    %\vspace{-10pt}
    \caption{\textbf{Visualization of spatio-temporal grounding on 3D tube.} The green tube is the GT box, and the line in the figure is the point with the max value in the attention heatmap.\label{fig:visual}}
\end{figure*}
